# Supplementary material for: Network Pruning Spaces
Source: arXiv:2304.09453 source file (2023-04-19)
Supplement: Supplementary file 1 [file appendix.tex]

% ==================
% ++++ Appendix ++++
% ==================
\newpage
\appendix

% ------------------
\section{MobileNetV2}

\input{floats/fig_std_spaces_flops_mob_v2_cifar10.tex}
\input{floats/fig_std_spaces_params_mob_v2_cifar10.tex}

\input{floats/fig_std_spaces_flops_r50_cifar10.tex}
\input{floats/fig_std_spaces_params_r50_cifar10.tex}

In this appendix we conduct experiments with \std pruning spaces for MobileNetV2.




% ------------------
\section{Implementation details}

In the appendix we provide details about training networks on CIFAR-10~\citep{krizhevsky2009learning} and ImageNet~\citep{russakovsky2015imagenet}.
We use the following settings if not specified: 4 GPUs and a batch size of 256 for both datasets; we optimize networks using SGD with a momentum of 0.9; we report the best accuracy observed.

\subsection{Pretraining networks}

\begin{table}[!h]
\centering
\caption{Pretraining networks on CIFAR-10 and ImageNet.
Results on CIFAR-10 are averaged over five runs.
In this table, \texttt{coslr} and \texttt{step} denote the cosine annealing schedule and step decay schedule respectively.}
\label{tab:pretraining}
\begin{tabular}{@{}cccccc@{}}
\toprule
Network & Dataset & Params & FLOPs & Schedule & Top-1 (\%) \\
\midrule
ResNet-50~\citep{he2016deep} & CIFAR-10 & 23.53M & 4.12G & \texttt{coslr} & $95.80 \pm 0.10$ \\
ResNet-50~\citep{he2016deep} & CIFAR-10 & 23.53M & 4.12G & \texttt{step}  & $95.41 \pm 0.20$ \\
ResNet-50~\citep{he2016deep} & ImageNet &        &       & \texttt{coslr} & 76.86 \\
ResNet-50~\citep{he2016deep} & ImageNet &        &       & \texttt{step}  & 76.86 \\
\bottomrule
\end{tabular}
\end{table}
